# Supplementary material for: Unified-IO 2: Scaling Autoregressive Multimodal Models with Vision, Language, Audio, and Action
Source: arXiv:2312.17172 source file (2023-12-28)
Supplement: Supplementary file 2 [file appendix_external_modules.tex]

\section{External Module}
\label{supp:external_module}

\subsection{VIT-VQGAN for Audio}
\label{supp:vit_vqgan}

\subsection{HiFi-GAN Vocoder}
\label{supp:hifi_gan}
