# Supplementary material for: Unified-IO 2: Scaling Autoregressive Multimodal Models with Vision, Language, Audio, and Action
Source: arXiv:2312.17172 source file (2023-12-28)
Supplement: Supplementary file 5 [file appendix_qualitative_results.tex]

\section{Qualitative results}
\label{supp:qualitative}

Additional qualitative examples are provided as a webpage in the supplementary materials.
